# Supplementary material for: Delayed luminescence and thermoluminescence in laboratory-grown diamonds
Source: arXiv:2407.11787 source file (2024-07-16)
Supplement: Supplementary file 1 [file Supplemental_information.pdf]

*Table: Summary of thermoluminescence glow peaks and activation energies of corresponding traps in various diamonds in the literature*

| Diamond              | Excitation    | $\beta$<br>(K/min) | Peak T<br>(K)                   | $E_A$ (eV)                         | Emission                           | Year [ref] |
|----------------------|---------------|--------------------|---------------------------------|------------------------------------|------------------------------------|------------|
| Type I<br>natural    | $\leq 300$ nm | -                  | 540                             | -                                  | “blue”                             | 1946 [15]  |
| Type I<br>industrial | 365 nm        | 150                | 420<br>520                      | 0.5<br>0.7                         | “blue”<br>“blue”                   | 1950 [16]  |
| Type I               | UV lamp       | 15                 | 180<br>330<br>525               | 0.12<br>0.4 – 0.5<br>1             | -<br>-<br>-                        | 1961 [17]  |
| Type IIa             |               |                    | 113<br>150<br>217<br>375<br>563 | 0.2<br>0.37<br>0.55<br>0.88<br>1.5 | -<br>-<br>-<br>-<br>-              |            |
| Type IIb             |               |                    | 140<br>250                      | 0.20<br>0.37                       | “blue”<br>“blue”                   |            |
| Type IIb             | $\geq 3$ eV   | 35                 | 150<br>260                      | 0.20<br>0.37                       | “blue”<br>“blue”                   | 1966 [18]  |
|                      | $\geq 1.8$ eV |                    | 175<br>285                      | 0.20<br>0.38                       | “red”<br>“red”                     |            |
| Type IIb             | $\geq E_g$    | 30                 | 150<br>250                      | 0.18(5)<br>0.35(2)                 | “red” / “blue”<br>1.85 eV/2.6 eV   |            |
| Type IIb             | Electrically  | 35                 | 265<br>280                      | -<br>-                             | “blue”<br>“red”                    | 1973 [19]  |
| Type IIb<br>Natural  | 4.88 eV       | 0.5 - 15           | 105<br>250<br>265<br>415        | 0.09<br>-<br>0.37(2)<br>0.8        | “red”<br>“red”<br>“blue”<br>“red”  | 1978 [20]  |
| Type IIb<br>HPHT     |               |                    | 105<br>210<br>265<br>320        | 0.09<br>0.22(2)<br>0.37(2)<br>0.38 | “red”<br>“blue”<br>“blue”<br>“red” |            |
| CVD film             | 200 – 400 nm  | 60                 | 336<br>563                      | 0.50 (3)<br>1.22 (6)               | 2.57 eV<br>“blue”                  | 2007 [21]  |
| Type IIa             | 224 nm        | 100                | -<br>-                          | 0.30(5)<br>0.37 (5)                | “blue”<br>“blue”                   | 2023 [12]  |

| Filter                       | Fluorescence                                                                      | Phosphorescence                                                                    |                                                                                     |
|------------------------------|-----------------------------------------------------------------------------------|------------------------------------------------------------------------------------|-------------------------------------------------------------------------------------|
|                              |                                                                                   | 0.1 s decay                                                                        | 5 s decay                                                                           |
| No filter                    | 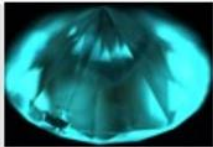 | 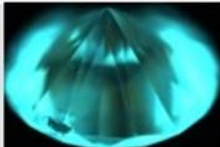 | 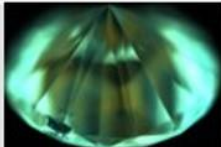 |
| Blue<br>(390 nm band pass)   | 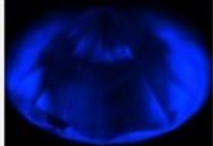 | 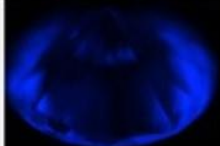 | 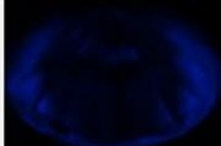 |
| Green<br>(475 nm long pass)  | 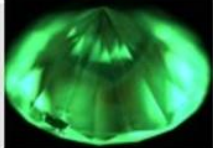 | 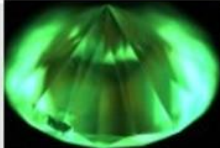 | 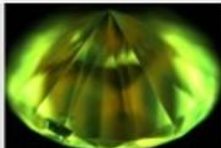 |
| Orange<br>(550 nm long pass) | 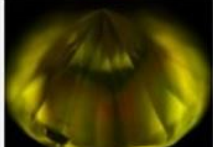 | 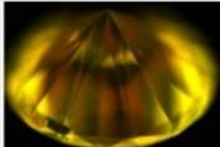 | 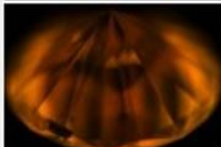 |

*Figure 1: DiamondView<sup>TM</sup> images of the Sino-01 sample. UV excited photoluminescence (fluorescence) and phosphorescence (0.1 s and 5 s delay time) with different filters at room temperature.*
